# Supplementary material for: Sets in homotopy type theory
Source: arXiv:1305.3835 source file (2014-04-24)
Supplement: Supplementary file 1 [file article-hsets-appendix.tex]

\section{The notion of a $\piw$-pretopos}\label{sec:pred_topos}

In this section we give the categorical definition of a $\piw$-pretopos; see \cite{johnstone:elephant}. There is one major difference 
between the notions of category
theory and our interpretations: where commuting diagrams of category theory commute with respect to extensional equality, we only require
diagrams in type theory to commute up to propositional equality.

\begin{defn}
Let $\mathcal{A}$ be a category with initial object and let $X,Y\in\mathcal{A}$ be objects for which the sum $X+Y$ exists. Then the sum
$X+Y$ is said to be \emph{disjoint} if the canonical maps $X\to X+Y$ and $Y\to X+Y$ are monomorphisms whose intersection is an initial
object.
\end{defn}

\begin{defn}
A category $\mathcal{A}$ is said to be \emph{lextensive} if it has finite limits and finite sums, where the sums are required to be disjoint  and stable under pullback.
\end{defn}

\begin{defn}
An epimorphism $e:a\to b$ is said to be \emph{regular} if it is the coequalizer of some pair $f,g:x\to a$ of morphisms.
\end{defn}

\begin{defn}
The \emph{kernel pair} of a morphism $f:A\to B$ is a pair $p_1,p_2:X\to A$ of morphisms such that the following diagram is a pullback.
\begin{equation*}
\begin{tikzcd}
X \ar{r}{p_1} \ar{d}[swap]{p_2} & A \ar{d}{f} \\
A \ar{r}[swap]{f} & B
\end{tikzcd}
\end{equation*}
\end{defn}

\begin{defn}
A category is said to be \emph{regular} if
\begin{enumerate}
\item it has all finite limits.
\item the kernel pair $(p_0,p_1)$ of any morphism $f$ has a coequalizer.
\item the pullback of a regular epimorphism along any morphism is again a regular epimorphism.
\end{enumerate}
\end{defn}

\begin{defn}
A morphism $f:A\to B$ is said to be a \emph{cover} if the only monomorphism (up to isomorphism) through which $f$ factors is $\idfunc{B}$.
\end{defn}

In a regular category, a morphism is a cover if and only if it is a regular epimorphism. Next we define what an exact category is. 

\begin{defn}
An \emph{equivalence relation} on an object $A$ is a subobject $(r_1,r_2):R\to A\times A$ for which
\begin{enumerate}
\item there is a morphism $\rho:A\to R$ such that $r_1\circ\rho=\idfunc{A}$ and $r_2\circ\rho=\idfunc{A}$.
\item there is a morphism $\sigma:R\to R$ such that $r_1\circ\sigma=r_2$ and $r_2\circ\sigma=r_1$. 
\item there is a morphism $\tau:R\times_A R\to R$ such that $r_1\circ\tau=r_1\circ\pi_1$ and $r_2\circ\tau=r_2\circ\pi_2$, where $\pi_1,\pi_2:R\times_A R\to R$ appear in the pullback diagram
\begin{equation*}
\begin{tikzcd}
R\times_A R \ar{r}{\pi_1} \ar{d}[swap]{\pi_2} & R \ar{d}{r_1} \\
R \ar{r}[swap]{r_2} & A
\end{tikzcd}
\end{equation*}
\end{enumerate}
\end{defn}

\begin{defn}
A morphism $f:A\to B$ is said to be a \emph{quotient} of an equivalence relation $(r_0,r_1)$ on $A$ if $f$ is the coequalizer of $r_0$ and $r_1$. 
\end{defn}

\begin{defn}
A relation $(r_1,r_2):R\to A\times A$ is said to be \emph{effective} if it is the kernel pair of its coequalizer.
\end{defn}

\begin{defn}
A category is said to be \emph{exact} if it is regular and every equivalence relation is effective. 
\end{defn}

\begin{defn}
A \emph{pretopos} is a category which is both exact and lextensive.
\end{defn}

\begin{defn}
A category $\mathcal{A}$ is said to be \emph{locally cartesian closed} if for any morphism $f:X\to Y$, the pullback functor
\begin{equation*}
f^\ast:\mathcal{A}/Y\to\mathcal{A}/X
\end{equation*}
has a right adjoint. Such a right adjoint is denoted by $\Pi_f$. 
\end{defn}

\begin{lem}
A category is locally cartesian closed if and only if all its slice categories are cartesian closed.
\end{lem}

\begin{defn}
A pretopos is said to be a \emph{$\Pi$-pretopos} if it is locally cartesian closed.
\end{defn}

\begin{defn}
Let $f:X\to Y$ is a morphism in a locally cartesian closed category $\mathcal{A}$. The polynomial functor $P_f$ associated to $f$ is the
endofunctor
\begin{equation*}
\begin{tikzcd}
\mathcal{A} \ar{r}{X\times{-}} & \mathcal{A}/X \ar{r}{\Pi_f} & \mathcal{A}/Y \ar{r}{\Sigma_f} & \mathcal{A}
\end{tikzcd}
\end{equation*}
An initial algebra for $P_f$ is called the \emph{$\mathsf{W}$-type} associated to $f$, or $\mathsf{W}_f$. The category $\mathcal{A}$ is said to have $\mathsf{W}$-types
if all the polynomial functors have initial algebras.
\end{defn}

\begin{defn}
A $\piw$-pretopos is a $\Pi$-pretopos which has $\mathsf{W}$-types.
\end{defn}
